# Supplementary material for: ReorderBench: A Benchmark for Matrix Reordering
Source: arXiv:2408.12169 source file (2025-04-10)
Supplement: Supplementary file 1 [file appendix-ref.tex]

@String(PAMI = {IEEE Trans. Pattern Anal. Mach. Intell.})
@String(IJCV = {Int. J. Comput. Vis.})
@String(CVPR= {IEEE Conf. Comput. Vis. Pattern Recognit.})
@String(ICCV= {Int. Conf. Comput. Vis.})
@String(ECCV= {Eur. Conf. Comput. Vis.})
@String(NIPS= {Adv. Neural Inform. Process. Syst.})
@String(ICPR = {Int. Conf. Pattern Recog.})
@String(BMVC= {Brit. Mach. Vis. Conf.})
@String(TOG= {ACM Trans. Graph.})
@String(TIP  = {IEEE Trans. Image Process.})
@String(TVCG  = {IEEE Trans. Vis. Comput. Graphics})
@String(TMM  = {IEEE Trans. Multimedia})
@String(ACMMM= {ACM Int. Conf. Multimedia})
@String(ICME = {Int. Conf. Multimedia and Expo})
@String(ICASSP=	{ICASSP})
@String(ICIP = {IEEE Int. Conf. Image Process.})
@String(ACCV  = {ACCV})
@String(ICLR = {Int. Conf. Learn. Represent.})
@String(ICML = {Int. Conf. Mach. Learn.})
@String(IJCAI = {IJCAI})
@String(PR   = {Pattern Recognition})
@String(AAAI = {AAAI})
@String(CVPRW= {IEEE Conf. Comput. Vis. Pattern Recog. Worksh.})
@String(CSVT = {IEEE Trans. Circuit Syst. Video Technol.})
@String(SPL	= {IEEE Sign. Process. Letters})
@String(VR   = {Vis. Res.})
@String(JOV	 = {J. Vis.})
@String(TVC  = {The Vis. Comput.})
@String(JCST  = {J. Comput. Sci. Tech.})
@String(CGF  = {Comput. Graph. Forum})
@String(CVM = {Computational Visual Media})

% articles
@article{kanizsa1976convexity,
  title={Convexity and symmetry in figure-ground orgnization},
  author={Kanizsa, Gaetano},
  journal={Vision and artifact},
  pages={25--32},
  year={1976},
}

@article{hilasaca2019overlap,
  author    = {Gladys M. H. Hilasaca and
               Fernando Vieira Paulovich},
  title     = {Distance Preserving Grid Layouts},
  journal   = {CoRR},
  volume    = {abs/1903.06262},
  year      = {2019},
  doi       = {10.48550/arXiv.1903.06262},
  url       = {http://arxiv.org/abs/1903.06262},
}

@article{frey2022optimizing,
  title={Optimizing Grid Layouts for Level-of-Detail Exploration of Large Data Collections},
  author={Frey, Steffen},
  journal=CGF,
  volume={41},
  number={3},
  pages={247--258},
  year={2022},
  doi = {10.1111/cgf.14537},
}

@article{fried2015isomatch,
  title={IsoMatch: Creating informative grid layouts},
  author={Fried, Ohad and DiVerdi, Stephen and Halber, Maciej and Sizikova, Elena and Finkelstein, Adam},
  journal=CGF,
  volume={34},
  number={2},
  pages={155--166},
  year={2015},
  doi = {10.1111/cgf.12549},
}

@article{strong2014self,
  title={Self-sorting map: An efficient algorithm for presenting multimedia data in structured layouts},
  author={Strong, Grant and Gong, Minglun},
  journal=TMM,
  volume={16},
  number={4},
  pages={1045--1058},
  year={2014},
  doi = {10.1109/TMM.2014.2306183}
}

@article{chen2020oodanalyzer,
  title={Oodanalyzer: Interactive analysis of out-of-distribution samples},
  author={Chen, Changjian and Yuan, Jun and Lu, Yafeng and Liu, Yang and Su, Hang and Yuan, Songtao and Liu, Shixia},
  journal=TVCG,
  volume={27},
  number={7},
  pages={3335--3349},
  year={2021},
  doi = {10.1109/TVCG.2020.2973258}
}

@article{rahtu2006new,
  title={A new convexity measure based on a probabilistic interpretation of images},
  author={Rahtu, Esa and Salo, Mikko and Heikkila, Janne},
  journal=PAMI,
  volume={28},
  number={9},
  pages={1501--1512},
  year={2006},
  doi = {10.1109/TPAMI.2006.175}
}

@article{rosin2006symmetric,
  title={A symmetric convexity measure},
  author={Rosin, Paul L and Mumford, Christine L},
  journal={Computer Vision and Image Understanding},
  volume={103},
  number={2},
  pages={101--111},
  year={2006},
  doi = {10.1016/j.cviu.2006.04.002}
}

@article{rosin2007probabilistic,
  title={Probabilistic convexity measure},
  author={Rosin, Paul L and {\v{Z}}uni{\'c}, Jovi{\v{s}}a},
  journal={IET image processing},
  volume={1},
  number={2},
  pages={182--188},
  year={2007},
  doi = {10.1049/iet-ipr:20060185}
}

@article{zunic2004new,
  title={A new convexity measure for polygons},
  author={\v{Z}uni\'{c}, Jovisa and Rosin, Paul L},
  journal=PAMI,
  volume={26},
  number={7},
  pages={923--934},
  year={2004},
  doi = {10.1109/TPAMI.2004.19}
}

@article{todorovic2008gestalt,
  title={Gestalt principles},
  author={Todorovic, Dejan},
  journal={Scholarpedia},
  volume={3},
  number={12},
  pages={5345},
  year={2008},
  doi={10.4249/scholarpedia.5345},
}

@article{liu2018correlatedmultiples,
  title={CorrelatedMultiples: Spatially Coherent Small Multiples With Constrained Multi-Dimensional Scaling},
  author={Liu, Xiaotong and Hu, Yifan and North, Stephen and Shen, Han-Wei},
  journal ={Computer Graphics Forum},
  volume={37},
  number={1},
  pages={7--18},
  year={2018},
  doi={10.1111/cgf.12526},
  organization={Wiley Online Library}
}

@article{barthel2022improved,
  title={Improved Evaluation and Generation Of Grid Layouts Using Distance Preservation Quality and Linear Assignment Sorting},
  author={Barthel, Kai Uwe and Hezel, Nico and Jung, Klaus and Schall, Konstantin},
  journal ={Computer Graphics Forum},
  year={2022},
  doi={10.1111/cgf.14718},
  organization={Wiley Online Library},
  note={to be published},
}

@article{lu2019winglets,
  title={Winglets: Visualizing association with uncertainty in multi-class scatterplots},
  author={Lu, Min and Wang, Shuaiqi and Lanir, Joel and Fish, Noa and Yue, Yang and Cohen-Or, Daniel and Huang, Hui},
  journal=TVCG,
  volume={26},
  number={1},
  pages={770--779},
  year={2020},
  doi={10.1109/TVCG.2019.2934811}
}

@article{rottmann2022mosaicsets,
  title={MosaicSets: Embedding Set Systems into Grid Graphs},
  author={Rottmann, Peter and Wallinger, Markus and Bonerath, Annika and Gedicke, Sven and N{\"o}llenburg, Martin and Haunert, Jan-Henrik},
  journal=TVCG,
  volume={29},
  number={1},
  pages={875--885},
  year={2023},
  doi={10.1109/TVCG.2022.3209485}
}

@article{dataset-mnist,
  title={Gradient-based learning applied to document recognition},
  author={LeCun, Yann and Bottou, L{\'e}on and Bengio, Yoshua and Haffner, Patrick},
  journal={Proceedings of the IEEE},
  volume={86},
  number={11},
  pages={2278--2324},
  year={1998},
  doi={10.1109/5.726791}
}

@article{dataset-usps,
  title={A database for handwritten text recognition research},
  author={Hull, Jonathan J.},
  journal=PAMI,
  volume={16},
  number={5},
  pages={550--554},
  year={1994},
  doi={10.1109/34.291440}
}

@article{wagemans2012century,
  title={A century of Gestalt psychology in visual perception: I. Perceptual grouping and figure-ground organization.},
  author={Wagemans, Johan and Elder, James H and Kubovy, Michael and Palmer, Stephen E and Peterson, Mary A and Singh, Manish and von der Heydt, R{\"u}diger},
  journal={Psychological bulletin},
  volume={138},
  number={6},
  pages={1172--1217},
  year={2012},
  doi={10.1037/a0029333}
}

@article{vzunic2019measuring,
  title={Measuring shapes with desired convex polygons},
  author={{\v{Z}}uni{\'c}, Jovi{\v{s}}a and Rosin, Paul L},
  journal=PAMI,
  volume={42},
  number={6},
  pages={1394--1407},
  year={2020},
  doi={10.1109/TPAMI.2019.2898830}
}


@article{bozeman2013convexity,
  title={The convexity ratio and applications},
  author={Bozeman, James R and Pilling, Matthew},
  journal={Scientiae Mathematicae Japonicae},
  volume={76},
  number={1},
  pages={47--53},
  year={2013},
  doi={10.32219/isms.76.1_47}
}

@article{huang2022conceptexplainer,
  title={ConceptExplainer: Interactive Explanation for Deep Neural Networks from a Concept Perspective},
  author={Huang, Jinbin and Mishra, Aditi and Kwon, Bum Chul and Bryan, Chris},
  journal=TVCG,
  volume={29},
  number={1},
  pages={831--841},
  year={2023},
  doi={10.1109/TVCG.2022.3209384}
}

@article{yuan2022visual,
  title={Visual Analysis of Neural Architecture Spaces for Summarizing Design Principles},
  author={Jun Yuan and Mengchen Liu and Fengyuan Tian and Shixia Liu},
  journal=TVCG,
  year = {2023},
  volume={29},
  number={1},
  pages={288--298},
  doi = {10.1109/TVCG.2022.3209404}
}

@article{yoghourdjian2015high,
  title={High-quality ultra-compact grid layout of grouped networks},
  author={Yoghourdjian, Vahan and Dwyer, Tim and Gange, Graeme and Kieffer, Steve and Klein, Karsten and Marriott, Kim},
  journal=TVCG,
  volume={22},
  number={1},
  pages={339--348},
  year={2016},
  doi={10.1109/TVCG.2015.2467251}
}

@article{eppstein2015improved,
  title={Improved grid map layout by point set matching},
  author={Eppstein, David and van Kreveld, Marc and Speckmann, Bettina and Staals, Frank},
  journal={International Journal of Computational Geometry \& Applications},
  volume={25},
  number={02},
  pages={101--122},
  year={2015},
  doi={10.1142/S0218195915500077}
}

@article{tu2022phrasemap,
  title={PhraseMap: Attention-Based Keyphrases Recommendation for Information Seeking},
  author={Tu, Yamei and Qiu, Rui and Wang, Yu-Shuen and Yen, Po-Yin and Shen, Han-Wei},
  journal=TVCG,
  year={2022},
  doi={10.1109/TVCG.2022.3225114},
  note={to be published},
}

@article{meulemans2016small,
  title={Small multiples with gaps},
  author={Meulemans, Wouter and Dykes, Jason and Slingsby, Aidan and Turkay, Cagatay and Wood, Jo},
  journal=TVCG,
  volume={23},
  number={1},
  pages={381--390},
  year={2017},
  doi={10.1109/TVCG.2016.2598542}
}

@article{pan2019content,
  title={Content-based visual summarization for image collections},
  author={Pan, Xingjia and Tang, Fan and Dong, Weiming and Ma, Chongyang and Meng, Yiping and Huang, Feiyue and Lee, Tong-Yee and Xu, Changsheng},
  journal=TVCG,
  volume={27},
  number={4},
  pages={2298--2312},
  year={2021},
  doi={10.1109/TVCG.2019.2948611}
}

@article{xia2022interactive,
  title={Interactive visual cluster analysis by contrastive dimensionality reduction},
  author={Xia, Jiazhi and Huang, Linquan and Lin, Weixing and Zhao, Xin and Wu, Jing and Chen, Yang and Zhao, Ying and Chen, Wei},
  journal=TVCG,
  volume={29},
  number={1},
  pages={734--744},
  year={2023},
  doi={10.1109/TVCG.2022.3209423}
}

@article{song2016gazedx,
  title={Gazedx: Interactive visual analytics framework for comparative gaze analysis with volumetric medical images},
  author={Song, Hyunjoo and Lee, Jeongjin and Kim, Tae Jung and Lee, Kyoung Ho and Kim, Bohyoung and Seo, Jinwook},
  journal=TVCG,
  volume={23},
  number={1},
  pages={311--320},
  year={2017},
  doi={10.1109/TVCG.2016.2598796}
}

@article{sevastjanova2022visual,
  title={Visual Comparison of Language Model Adaptation},
  author={Sevastjanova, Rita and Cakmak, Eren and Ravfogel, Shauli and Cotterell, Ryan and El-Assady, Mennatallah},
  journal=TVCG,
  volume={29},
  number={1},
  pages={1178--1188},
  year={2023},
  doi={10.1109/TVCG.2022.3209458}
}

@article{felix2016texttile,
  title={TextTile: An interactive visualization tool for seamless exploratory analysis of structured data and unstructured text},
  author={Felix, Cristian and Pandey, Anshul Vikram and Bertini, Enrico},
  journal=TVCG,
  volume={23},
  number={1},
  pages={161--170},
  year={2017},
  doi={10.1109/TVCG.2016.2598447}
}

@article{choi2021dxplorer,
  title={DXplorer: a unified visualization framework for interactive dendritic spine analysis using 3D morphological features},
  author={Choi, Junyoung and Lee, Sang-Eun and Lee, Yein and Cho, Eunji and Chang, Sunghoe and Jeong, Won-Ki},
  journal=TVCG,
  volume={29},
  number={2},
  pages={1424--1437},
  year={2023}
}

@article{chan2019motion,
  title={Motion Browser: visualizing and understanding complex upper limb movement under obstetrical brachial plexus injuries},
  author={Chan, Gromit Yeuk-Yin and Nonato, Luis Gustavo and Chu, Alice and Raghavan, Preeti and Aluru, Viswanath and Silva, Cl{\'a}udio T},
  journal=TVCG,
  volume={26},
  number={1},
  pages={981--990},
  year={2020},
  doi={10.1109/TVCG.2019.2934280}
}

@article{keefe2009interactive,
  title={Interactive coordinated multiple-view visualization of biomechanical motion data},
  author={Keefe, Daniel and Ewert, Marcus and Ribarsky, William and Chang, Remco},
  journal=TVCG,
  volume={15},
  number={6},
  pages={1383--1390},
  year={2009},
  doi={10.1109/TVCG.2009.152}
}

@article{oppermann2021vizsnippets,
  title={VizSnippets: Compressing Visualization Bundles Into Representative Previews for Browsing Visualization Collections},
  author={Oppermann, Michael and Munzner, Tamara},
  journal=TVCG,
  volume={28},
  number={1},
  pages={747--757},
  year={2022},
  doi={10.1109/TVCG.2021.3114841}
}

@article{major2018graphicle,
  title={Graphicle: Exploring units, networks, and context in a blended visualization approach},
  author={Major, Timothy and Basole, Rahul C},
  journal=TVCG,
  volume={25},
  number={1},
  pages={576--585},
  year={2019},
  doi={10.1109/TVCG.2018.2865151}
}

@article{zeng2020revisiting,
  title={Revisiting the modifiable areal unit problem in deep traffic prediction with visual analytics},
  author={Zeng, Wei and Lin, Chengqiao and Lin, Juncong and Jiang, Jincheng and Xia, Jiazhi and Turkay, Cagatay and Chen, Wei},
  journal=TVCG,
  volume={27},
  number={2},
  pages={839--848},
  year={2021},
  doi={10.1109/TVCG.2020.3030410}
}

@article{yang2022epimob,
  title={Epimob: Interactive visual analytics of citywide human mobility restrictions for epidemic control},
  author={Yang, Chuang and Zhang, Zhiwen and Fan, Zipei and Jiang, Renhe and Chen, Quanjun and Song, Xuan and Shibasaki, Ryosuke},
  journal=TVCG,
  year={2022},
  doi={10.1109/TVCG.2022.3165385},
  note={to be published}
}

@article{vandenhende2021multi,
  title={Multi-task learning for dense prediction tasks: A survey},
  author={Vandenhende, Simon and Georgoulis, Stamatios and Van Gansbeke, Wouter and Proesmans, Marc and Dai, Dengxin and Van Gool, Luc},
  journal=PAMI,
  volume={44},
  number={7},
  pages={3614--3633},
  year={2022},
  doi={10.1109/TPAMI.2021.3054719}
}

@article{held1994approximate,
  title={On approximate convexity},
  author={Held, Andreas and Abe, Keiichi},
  journal={Pattern recognition letters},
  volume={15},
  number={6},
  pages={611--618},
  year={1994},
  doi={10.1016/0167-8655(94)90022-1}
}

@article{song2021balance,
  title={Balance-aware grid collage for small image collections},
  author={Song, Yu and Tang, Fan and Dong, Weiming and Huang, Feiyue and Lee, Tong-Yee and Xu, Changsheng},
  journal=TVCG,
  volume={29},
  number={2},
  pages={1330--1344},
  year={2023},
  doi={10.1109/TVCG.2021.3113031}
}
% articles end


% inproceeding
@inproceedings{deng2009imagenet,
  title={Imagenet: A large-scale hierarchical image database},
  author={Deng, Jia and Dong, Wei and Socher, Richard and Li, Li-Jia and Li, Kai and Fei-Fei, Li},
  booktitle={CVPR},
  pages={248--255},
  year={2009},
  doi={10.1109/CVPR.2009.5206848},
}

@inproceedings{schoeffmann2011similarity,
  title={Similarity-based visualization for image browsing revisited},
  author={Schoeffmann, Klaus and Ahlstrom, David},
  booktitle={2011 IEEE International Symposium on Multimedia},
  pages={422--427},
  year={2011},
  doi={10.1109/ISM.2011.76},
  organization={IEEE}
}

@inproceedings{yang2020diagnosing,
  title={Diagnosing Concept Drift with Visual Analytics},
  author={Yang, Weikai and Li, Zhen and Liu, Mengchen and Lu, Yafeng and Cao, Kelei and Maciejewski, Ross and Liu, Shixia},
  booktitle={{IEEE} Conference on Visual Analytics Science and Technology},
  pages={12--23},
  year={2020},
  doi={10.1109/VAST50239.2020.00007}
}

@inproceedings{efrat2014mapsets,
  title={MapSets: Visualizing embedded and clustered graphs},
  author={Efrat, Alon and Hu, Yifan and Kobourov, Stephen G and Pupyrev, Sergey},
  booktitle={Graph Drawing: 22nd International Symposium, GD 2014, W{\"u}rzburg, Germany, September 24-26, 2014, Revised Selected Papers 22},
  pages={452--463},
  year={2014},
  doi={10.1007/978-3-662-45803-7_38},
  organization={Springer}
}

@inproceedings{bruls2000squarified,
  title={Squarified treemaps},
  author={Bruls, Mark and Huizing, Kees and Van Wijk, Jarke J},
  booktitle={Data Visualization 2000: Proceedings of the Joint EUROGRAPHICS and IEEE TCVG Symposium on Visualization in Amsterdam, The Netherlands, May 29--30, 2000},
  pages={33--42},
  year={2000},
  doi={10.1007/978-3-7091-6783-0_4},
  organization={Springer}
}

@inproceedings{luboschik2010new,
  title={A new weaving technique for handling overlapping regions},
  author={Luboschik, Martin and Radloff, Axel and Schumann, Heidrun},
  booktitle={Proceedings of the International Conference on Advanced Visual Interfaces},
  pages={25--32},
  doi={10.1145/1842993.1842999},
  year={2010}
}

@inproceedings{matejka2018dream,
  title={Dream lens: Exploration and visualization of large-scale generative design datasets},
  author={Matejka, Justin and Glueck, Michael and Bradner, Erin and Hashemi, Ali and Grossman, Tovi and Fitzmaurice, George},
  booktitle={Proceedings of the 2018 CHI conference on human factors in computing systems},
  pages={1--12},
  doi={10.1145/3173574.3173943},
  year={2018}
}

@inproceedings{rote2013degree,
  title={The degree of convexity},
  author={Rote, G{\"u}nter},
  booktitle={29th European Workshop on Computational Geometry},
  pages={69--72},
  year={2013}
}

@inproceedings{halnaut2022vrgrid,
  title={VRGrid: Efficient Transformation of 2D Data into Pixel Grid Layout},
  author={Halnaut, Adrien and Giot, Romain and Bourqui, Romain and Auber, David},
  booktitle={26th International Conference Information Visualisation},
  year={2022}
}

@inproceedings{peura1997efficiency,
  title={Efficiency of simple shape descriptors},
  author={Peura, Markus and Iivarinen, Jukka and others},
  booktitle={Proceedings of the third international workshop on visual form},
  pages={443--451},
  year={1997}
}

@inproceedings{radford2021learning,
  title={Learning transferable visual models from natural language supervision},
  author={Radford, Alec and Kim, Jong Wook and Hallacy, Chris and Ramesh, Aditya and Goh, Gabriel and Agarwal, Sandhini and Sastry, Girish and Askell, Amanda and Mishkin, Pamela and Clark, Jack and Krueger, Gretchen and Sutskever, Ilya},
  booktitle={Proceedings of the 38th International Conference on Machine Learning},
  pages={8748--8763},
  year={2021},
  organization={PMLR},
  pdf={http://proceedings.mlr.press/v139/radford21a/radford21a.pdf},
  url={https://proceedings.mlr.press/v139/radford21a.html}
}

@inproceedings{chen2018gradnorm,
  title={{G}rad{N}orm: Gradient Normalization for Adaptive Loss Balancing in Deep Multitask Networks},
  author={Chen, Zhao and Badrinarayanan, Vijay and Lee, Chen-Yu and Rabinovich, Andrew},
  booktitle={Proceedings of the 35th International Conference on Machine Learning},
  pages={794--803},
  year={2018},
  organization={PMLR},
  pdf={http://proceedings.mlr.press/v80/chen18a/chen18a.pdf},
  url={https://proceedings.mlr.press/v80/chen18a.html}
}

@inproceedings{quadrianto2008kernelized,
 author = {Quadrianto, Novi and Song, Le and Smola, Alex},
 booktitle = {Advances in Neural Information Processing Systems},
 editor = {D. Koller and D. Schuurmans and Y. Bengio and L. Bottou},
 pages = {},
 title = {Kernelized Sorting},
 url = {https://proceedings.neurips.cc/paper/2008/file/94c7bb58efc3b337800875b5d382a072-Paper.pdf},
 year = {2008}
}
% end inproceeding 
% books
@book{sonka2014image,
  title={Image processing, analysis, and machine vision},
  author={Sonka, Milan and Hlavac, Vaclav and Boyle, Roger},
  year={2014},
  publisher={Cengage Learning}
}

@book{munzner2014visualization,
  title={Visualization analysis and design},
  author={Munzner, Tamara},
  year={2014},
  publisher={CRC press}
}

@book{do2016differential,
  title={Differential geometry of curves and surfaces: revised and updated second edition},
  author={Do Carmo, Manfredo P},
  year={2016},
  publisher={Courier Dover Publications}
}

@incollection{barthel2019visually,
  doi = {10.1002/9781119376996.ch11},
  url = {https://doi.org/10.1002/9781119376996.ch11},
  year = {2019},
  month = mar,
  publisher = {John Wiley {\&} Sons,  Ltd},
  pages = {289--315},
  author = {Kai Uwe Barthel and Nico Hezel},
  title = {Visually Exploring Millions of Images using Image Maps and Graphs},
  booktitle = {Big Data Analytics for Large-Scale Multimedia Search}
}
% end books

% others
@misc{tsnegrid,
  title = {Image t-{SNE} {Live}},
  howpublished = {\url{https://ml4a.github.io/guides/ImageTSNELive/}},
  year={2016},
  note = "Last accessed 2023-3-31"
}

@misc{dataset-animals,
  title = {{Animals-10 dataset}},
  author = {{A}. {C}orrado},
  howpublished = {\url{https://www.kaggle.com/datasets/alessiocorrado99/animals10/}},
  year={2019},
  note = "Last accessed 2023-3-31"
}

@techreport{dataset-cifar10,
  title={Learning multiple layers of features from tiny images},
  author={A. Krizhevsky and G. Hinton},
  year={2009},
  institution={University of Toronto, Toronto, Ontario}
}

@techreport{johnson1998tree,
  title={Tree-maps: A space filling approach to the visualization of hierarchical information structures},
  author={Johnson, Brian and Shneiderman, Ben},
  year={1998}
}
@article{Liu_Liang_Gitter_2019,
title={Loss-Balanced Task Weighting to Reduce Negative Transfer in Multi-Task Learning},
volume={33},
doi={10.1609/aaai.v33i01.33019977},
number={01},
journal={Proceedings of the AAAI Conference on Artificial Intelligence},
author={Liu, Shengchao and Liang, Yingyu and Gitter, Anthony},
year={2019},
pages={9977-9978}
}
@article{collins2009bubble,
  title={Bubble sets: Revealing set relations with isocontours over existing visualizations},
  author={Collins, Christopher and Penn, Gerald and Carpendale, Sheelagh},
  journal=TVCG,
  volume={15},
  number={6},
  pages={1009--1016},
  year={2009},
  doi={10.1109/TVCG.2009.122},
}
@article{breiman1996bagging,
  title={Bagging predictors},
  author={Breiman, Leo},
  journal={Machine learning},
  volume={24},
  pages={123--140},
  year={1996},
  doi={10.1007/BF00058655}
}
